# Supplementary material for: The Spectrum of Fisher Information of Deep Networks Achieving Dynamical Isometry
Source: arXiv:2006.07814 source file (2021-03-29)
Supplement: Supplementary file 1 [file appendix_free_back.tex]

\section{Free Probability Theory for ML }

\newcommand{\C}{{\mathbb{C}}}

\paragraph{Random Matrix Model}

\paragraph{Asymptotic Freeness}

The free $\C$-algebra on $n$ indeterminate $X_1, \dots, X_n$ is the 
\begin{defn}
$\C \langle X \rangle$
\end{defn}

\paragraph{Infinite Dimensional Approximation}

We consider the infinite dimensional approximation $M \to \infty$.
Under the assumption of asymptotic freeness, we consider the following assumption.
\paragraph{Free Model}
Let $(\mathfrak{A},\tau)$ be a C$^*$-probability space.
Let $L \in \N$ with $L \geq 2$.
\begin{enumerate}
    \item  $ \fda_\ell \in \mathfrak{A}_{s.a.}$ $(\ell=1, \dots , L-1)$
     \item $w_1, \dots,w_L \in \mathfrak{A} $ are  scaled Haar unitaries.
    \item $ (\{\fda_1, \dots, \fda_{L-1} \}, \{w_2, w_2^*\}, \dots, \{w_L, w_L^*\} )$ is free.
\end{enumerate}

We define \emph{free error} by 
\begin{align}
\delta_{L \to \ell}^\Box := \begin{cases} w_L \fda_{L-1} \dots  w_{\ell+1} \fda_\ell  &; \ell <L,\\
1 &; \ell=L.
\end{cases}
\end{align}
If there is no confusion, we simply write $\delta^\Box_\ell$.
As the finite dimensional case, we have  the following back-propagation of free error ;
\begin{align}
    \fdelta_\ell =  \fdelta_{\ell + 1} w_{\ell+1} \fda_{\ell}.
\end{align}

Write scalars:
\begin{enumerate}
    \item  $ \sigma_{w, \ell}^2 :=  \tau(w_\ell w_\ell^*) > 0$.
    \item  $q_\ell \in \R, q_\ell > 0$
\end{enumerate}

We define \emph{the free neural tangent kernel} by 
\begin{align}
   \FNTK_L:=  \sum_{\ell=1}^L q_{\ell-1} \fdelta_\ell (\fdelta_\ell)^*.
\end{align}

Note that
\begin{align}
    \tau(\FNTK_L) =  \sum_{\ell=1}^L q_{\ell-1} \tilde{q}_{\ell}.
\end{align}

For $\ell < L$, 
\begin{align}
    \delta_{L \to \ell}  = w_L a_{L-1} \delta_{L-1 \to \ell}.
\end{align}

\begin{lemma}
\begin{align}
    \FNTK_L &=   q_{L-1} +  \sum_{\ell=1}^{L-1} w_L a_{L-1} \fdelta_{L-1 \to \ell} (\fdelta_{L-1 \to \ell})^* a_{L-1} w_L^*\\
    &= q_{L-1} +  w_L a_{L-1}\FNTK_{L-1} a_{L-1} w_L^*
\end{align}
\end{lemma}

\subsection{ReLU-like activation}
Assume  each $a_\ell$ be a scaled projection. Write
\begin{align}
    a_\ell &= \sqrt{\gamma_\ell} p_\ell\\
    \alpha_\ell &:= \tau(p_\ell)
\end{align}
Write
\begin{align}
    u_\ell &:=  w_\ell / \sigma_{w,\ell}\\
    \sigma_\ell^2  &= v_{w,\ell+1} \gamma_\ell
\end{align}

Then
\begin{align}
    \delta_\ell = \delta_{\ell+1} ( \sigma_\ell u_{\ell+1}p_{\ell} )
\end{align}

\begin{align}
    \FNTK_L = q_{L-1} +  \sigma_L^2  u_L p_{L-1}\FNTK_{L-1} p_{L-1} u_L^*
\end{align}

\begin{thm}
\begin{align}
    \mu_{\FNTK_L} =   \delta_{q_{L-1}} \boxplus   (  \delta_{\sigma_L^2}  \boxtimes \mu_{ p_{L-1}}  \boxtimes \mu_{\FNTK_{L-1}} )
\end{align}
\end{thm}

\subsection{Normalization}
Consider
\begin{align}
    \tilde{\FNTK}_L := \FNTK_L/q_{L-1}.
\end{align}
For $L>1$,
\begin{align}
    \tilde{\FNTK}_L =   1   +  \frac{\sigma_L^2 q_{L-2}}{q_{L-1} } u_L p_{L-1}\tilde{\FNTK}_{L-1} p_{L-1} u_L^* 
\end{align}
Write 
\begin{align}
    r_{L} &:=    \sigma_{L} \frac{q_{L-2}}{q_{L-1}},
\end{align}
for $L>2$, and $r_1 := 0$. Then
\begin{align}
    \tilde{\FNTK}_L =   1   +  r_L u_L p_{L-1}\tilde{\FNTK}_{L-1} p_{L-1} u_L^* 
\end{align}
